# Supplementary material for: Predictive Visuo-Tactile Interactive Perception Framework for Object Properties Inference
Source: arXiv:2411.09020 source file (2024-11-13)
Supplement: Supplementary file 1 [file appendix_old.tex]

\section{Appendix}
\subsection{Mechanics of object-robot interaction}
Objects with single link and uniform properties have an analytical model of quasi-static pushing that was created by Lynch et al. \cite{lynch1992manipulation}. This model is based on several assumptions, but it helps to comprehend which physical parameters are involved in non-prehensile pushing. After a thorough review, no work that used the analytical model for parameter estimation was found; therefore, this provided a scope of research. We provide extensive results on parameter estimation using the analytical model in the results section. 

\subsubsection*{Analytical model of non-prehensile pushing}
The analytical model of quasi-static pushing predicts object movement $v_t$, given the robot pushing velocity $(u)$, the contact point $(cp)$, and associated surface normal at the contact point $n$, as well as surface friction $\mu$ and friction between the object and the robot $\mu_r$. Predicting the effect of the push with this model has two stages. 

First, we determine whether the contact between the object and the robot is slipping or sticking, and then we compute the effective push velocity. 


\begin{figure}[t!]
    \centering
    \includegraphics[width=0.9\columnwidth]{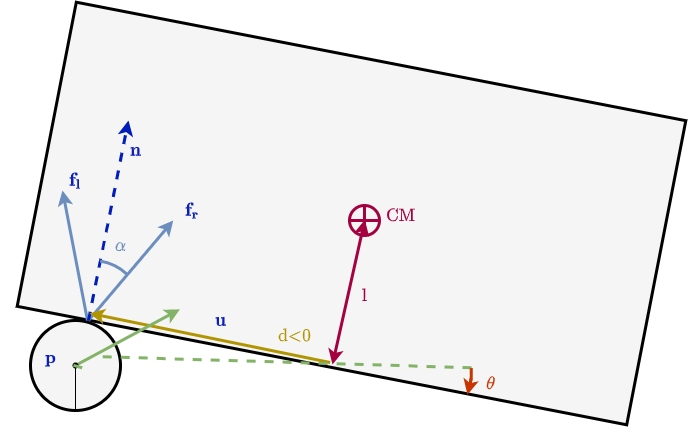}
    \caption{Analytical model of planar pushing}
    \label{fig:push_anal}
\end{figure}


\begin{align}
    & \alpha = arctan(\mu_r) \\
    & \mathbf{f_l} = \mathbf{R}(-\alpha)\mathbf{n} \\
    & \mathbf{f_r} = \mathbf{R}(\alpha)\mathbf{n} \\
    & m_l = cp_{x}f_{ly}-cp_{y}f_{lx} \\
    & m_r = c_{x}f_{ry}-c_{y}f_{rx}
\end{align}

The rotation matrix $\mathbf{R}(\alpha)$ represents a rotation about the $z$-axis with an angle $\alpha$. The contact point $cp$ and the surface normal $\mathbf{n}$ are relative to the center of mass of the object. Lynch et al. \cite{lynch1992manipulation} used an ellipsoidal approximation of the limit surface to relate the forces to the velocities of the object. To simplify the notation, the subscript $b$ is used to refer to either the left ($l$) or right ($r$) boundary forces. The linear and angular object velocities are denoted by $v_{o,b}$ and $\omega_{o,b}$, respectively. The push velocities that would be created from the boundary forces are referred to as $v_{p,b}$ and form the so-called "motion cone" as shown in Figure.\ref{}.

\begin{align}
  & v_{o,b} = \frac{\omega_{o, b}l^2}{m_b}f_b \\
  & v_{p,b} = \omega_{o, b}(\frac{l^2}{m_b}f_b + k \times cp) 
\end{align}

Here, $k$ is the rotation of the object. where $\omega_{o,b}$ acts as a scaling factor. As we are only interested in the direction of $v_{p,b}$ and not in its magnitude, we set $\omega_{o,b}=m_b$:

\begin{equation}
     v_{p,b} = l^2f_b + m_b k \times c^{'}
\end{equation}

To compute the effective push velocity $v_p$, we need to determine the contact case: if the push velocity lies outside the motion cone, the contact will slip. The resulting effective push then acts in the direction of the boundary velocity $v_{p,b}$, which is closer to the push direction:

\begin{equation}
     v_{p} = \frac{u n}{v_{p,b} n} v_{p,b}
\end{equation}

Otherwise, the contact sticks and we can use the pusher velocity as the effective push velocity $v_p = u$. Now given the effective push velocity in both sticking and slipping case, we can compute the linear and angular velocity $v_o=[v_{ox}, v_{oy}, \omega]$

\begin{align}
    & v_{ox} = \frac{(l^{2} + c^{'2}_{x})v_{px} + c^{'}_{x} c^{'}_{y}}{l^{2} + c^{'2}_{x} + c^{'2}_{y}}v_{px} \\
    & v_{oy} = \frac{(l^{2} + c^{'2}_{x})v_{px} + c^{'}_{x} c^{'}_{y}}{l^{2} + c^{'2}_{x} + c^{'2}_{y}}v_{px} \\
    & \omega = \frac{c^{'}_{x} v_{oy} - c^{'}_{y} v_{ox}}{l^{2}}
\end{align}

%The interaction dynamics gets even more difficult to model for non-homogenous objects and articulated objects. In addition, the presented analytical model has certain assumptions, which is violated. Therefore, we resort to data. However, based on the best review, we have not found any works which have utilised the model for parameter estimation, and therefore interesting to compare to. As a first step to make it generalizable, it is essential to infer the shape of the object. %\textcolor{red}{add why prehensile pull is skipped, good explanation, add some analysis terms}.



\section{Additional results}
\subsection{Qualitative shape perception results}
Here is the plot for all the shapes considered in the works, the noisey point cloud after multiple views, superquadric shape estimated and the overlayed visualization for better illustration. We can observe the shape represents the actual object quite well, sufficient for table top pushing and pulling. 

\begin{figure*}[!htb]
    \centering
    \includegraphics[width = \textwidth]{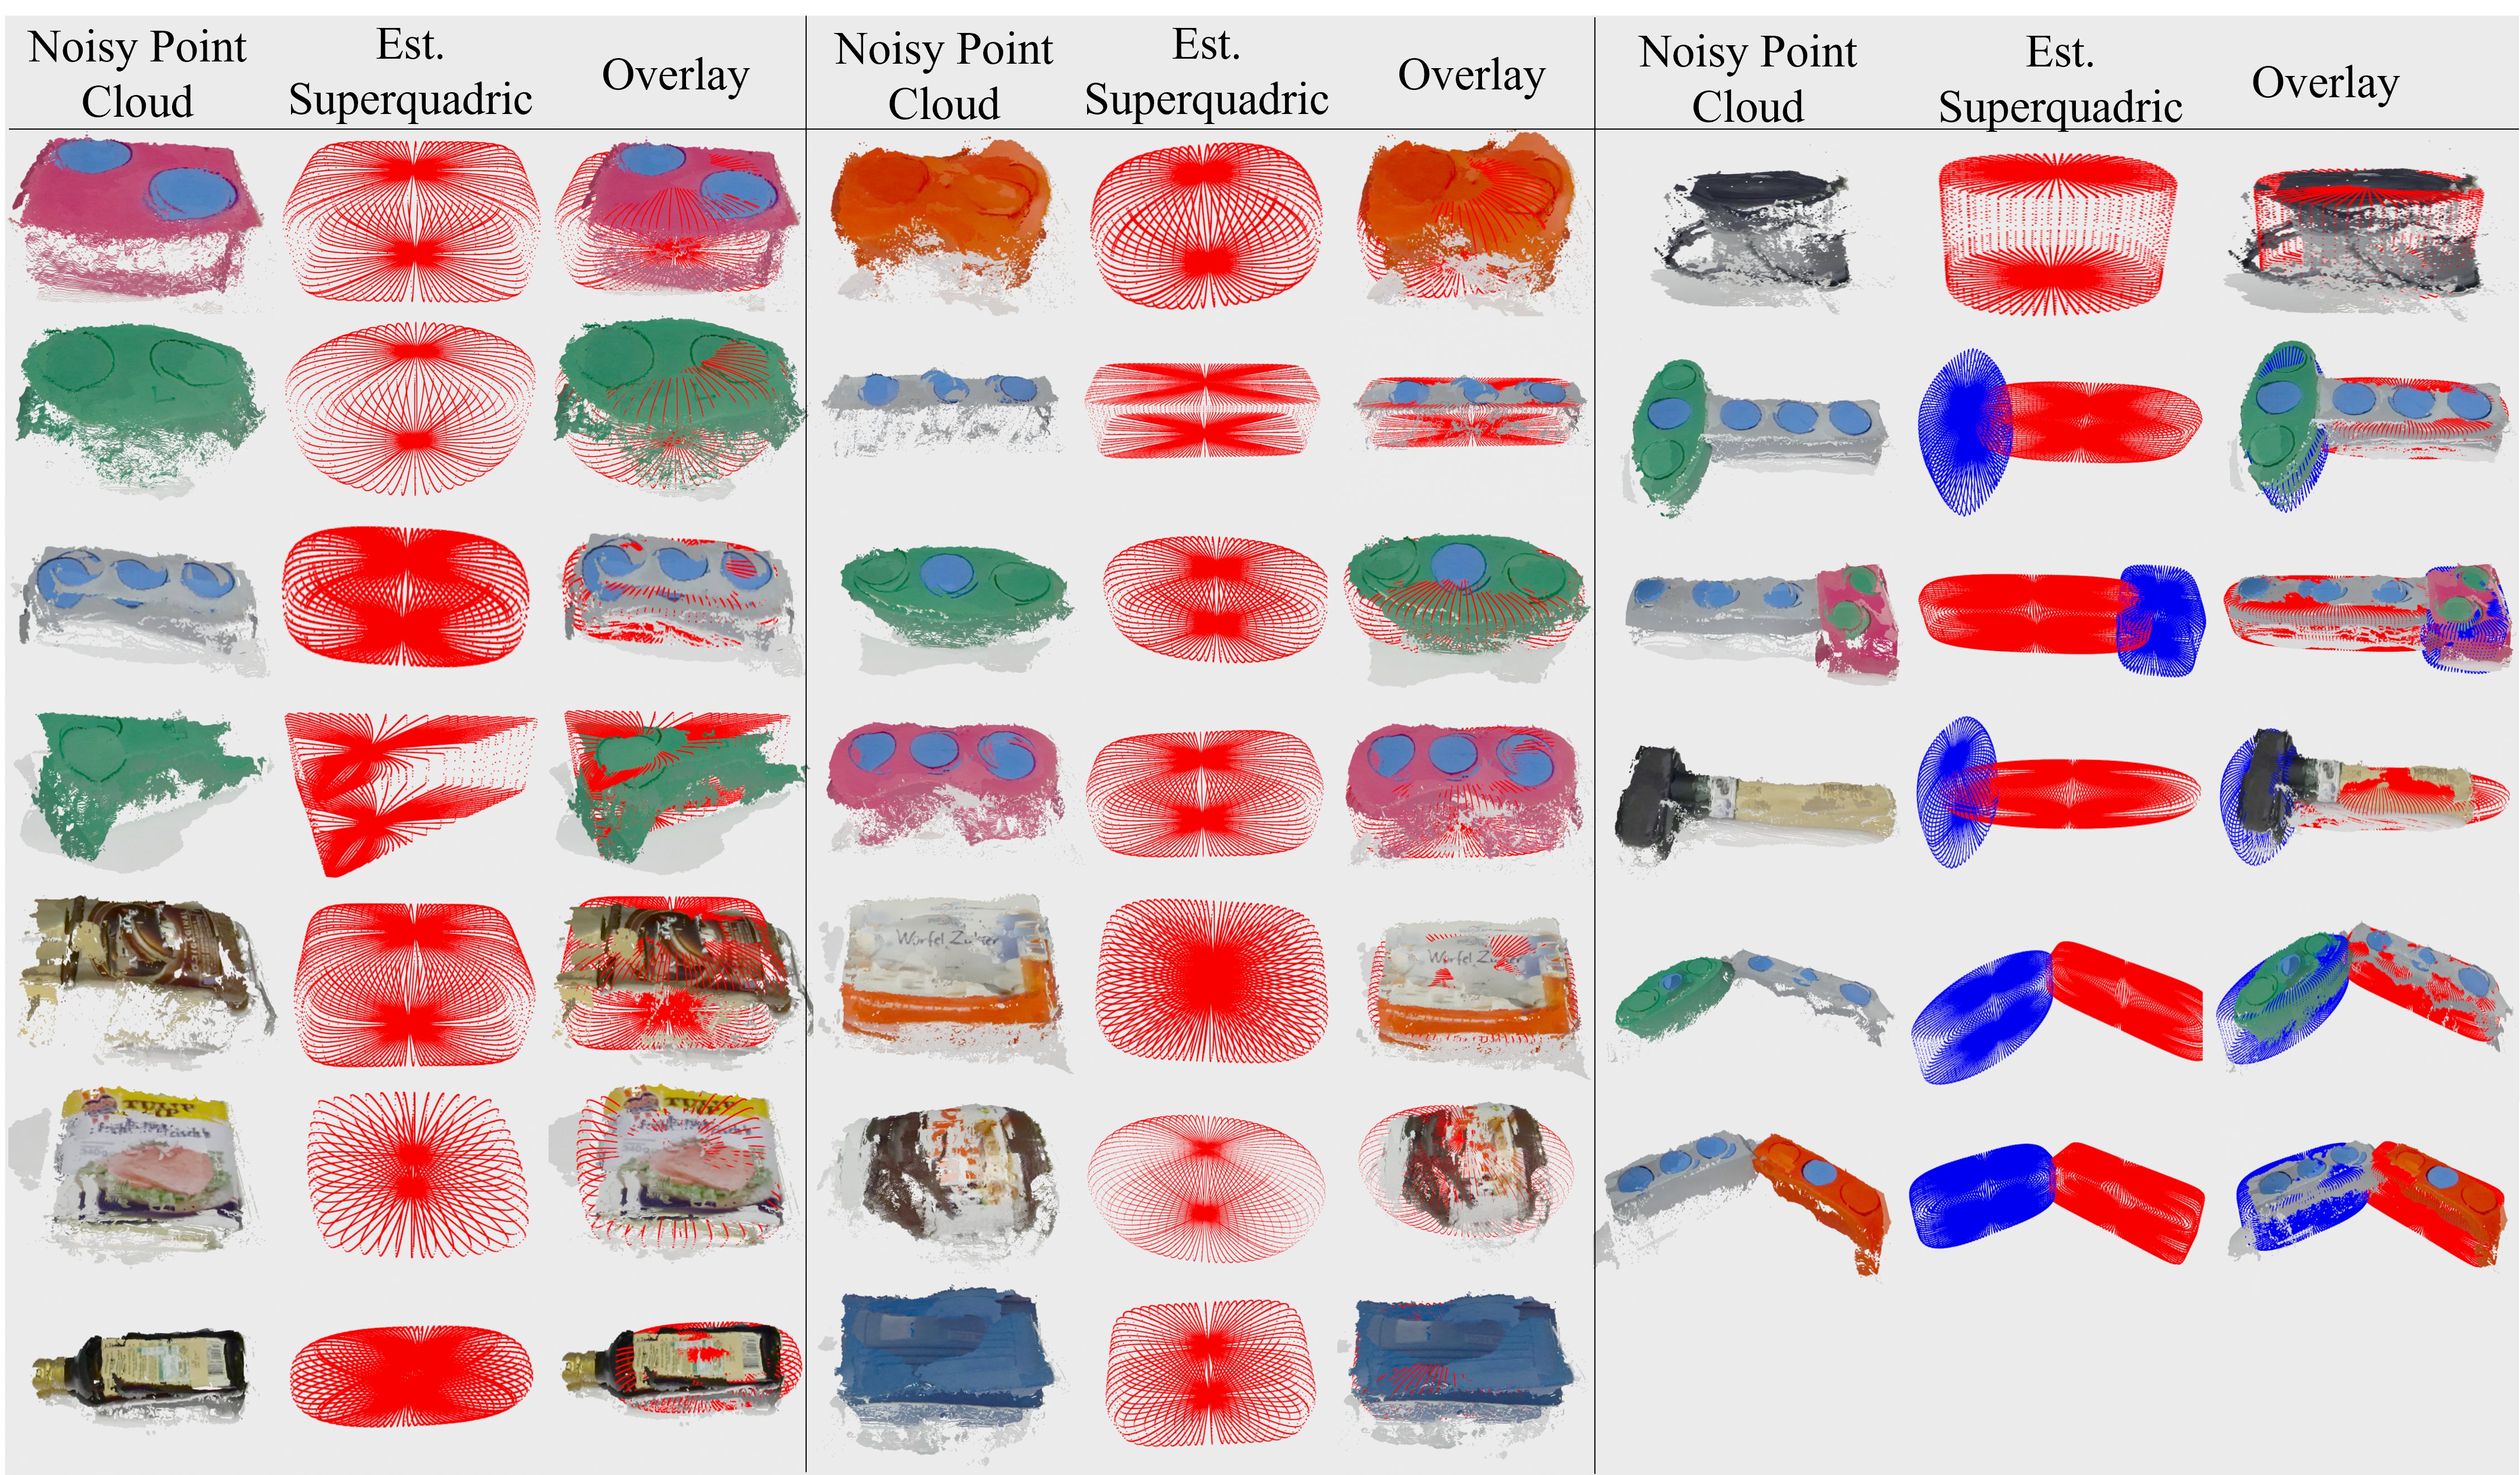}
    \caption{Shape result perception result of 3D configurable objects and daily objects}
    \label{fig:qualshapeplot}
\end{figure*}

\subsection{Model prediction}
We also illustrative pose prediction and tactile prediction of the trained models for a validation object. This is done without utilizing the differentiable filter (only using the prediction step), as shown in Fig. \ref{fig:validationplotuni}, Fig.\ref{fig:validationplotheter}, and Fig.\ref{fig:validationplotart} for \textit{homogeneous}, \textit{heterogeneous}, and \textit{articulated} objects, respectively. It can be observed that the $GNN$ model is able to capture the stochastic dynamics and complexity of the tactile sensor embodiment more effectively in the case of homogeneous objects compared to $Analytical$. Furthermore, it outperforms the $FF$ model in the context of interactions with heterogeneous and articulated objects. It is also evident that the prediction has significant errors that require the filtering process.

\begin{figure}[ht!]
    \centering
    \includegraphics[width = \columnwidth]{figures/results/pred_plot_uniform.png}
    \caption{Validation results of the homogeneous object trajectory prediction without filtering a) and b) are both push actions}
    \label{fig:validationplotuni}
\end{figure}

\begin{figure}[ht!]
    \centering
    \includegraphics[width = \columnwidth]{figures/results/pred_plot_hetero.png}
    \caption{Validation results of the heterogeneous object trajectory prediction without filtering a) is push action whereas b) is pull action.}
    \label{fig:validationplotheter}
\end{figure}

\begin{figure}[ht!]
    \centering
    \includegraphics[width = \columnwidth]{figures/results/pred_plot_art.png}
    \caption{Validation results of the articulated object trajectory prediction without filtering a) is push action whereas b) is pull action.}
    \label{fig:validationplotart}
\end{figure}


%%%%%%%%%%%%%%%%%%%%%%%% Filtering %%%%%%%%%%%%%%%%%%%
\subsection{Dual Differentiable Filtering}
Fig. \ref{fig:filteringuniform} illustrates a detailed examination of the dual filtering process using the $Active-GNN$ approach. The plots show the filtering of pose and parameter state of a representative test case that involving a \textit{homogeneous} object with a non-prehensile pushing trajectory for exploration. Similarly, Figs. \ref{fig:filteringheteropush} and \ref{fig:filteringheteropull} depict the filtering procedure for a \textit{heterogeneous} object with non-prehensile pushing and prehensile pulling, respectively. Additionally, Figs. \ref{fig:filteringarticulatedpush} and \ref{fig:filteringarticulatedpull} present the filtering outcome for an \textit{articulated} object. These plots provide insights into the evolution of parameter variance over time and its impact on object pose estimation and filtering. The ground truth pose and the parameter are denoted as $GT$.

This filtering process is carried out over multiple interactions until the variance over the parameters is reduced.

\begin{figure*}[!tbh]
    \centering
    \includegraphics[width = \textwidth]{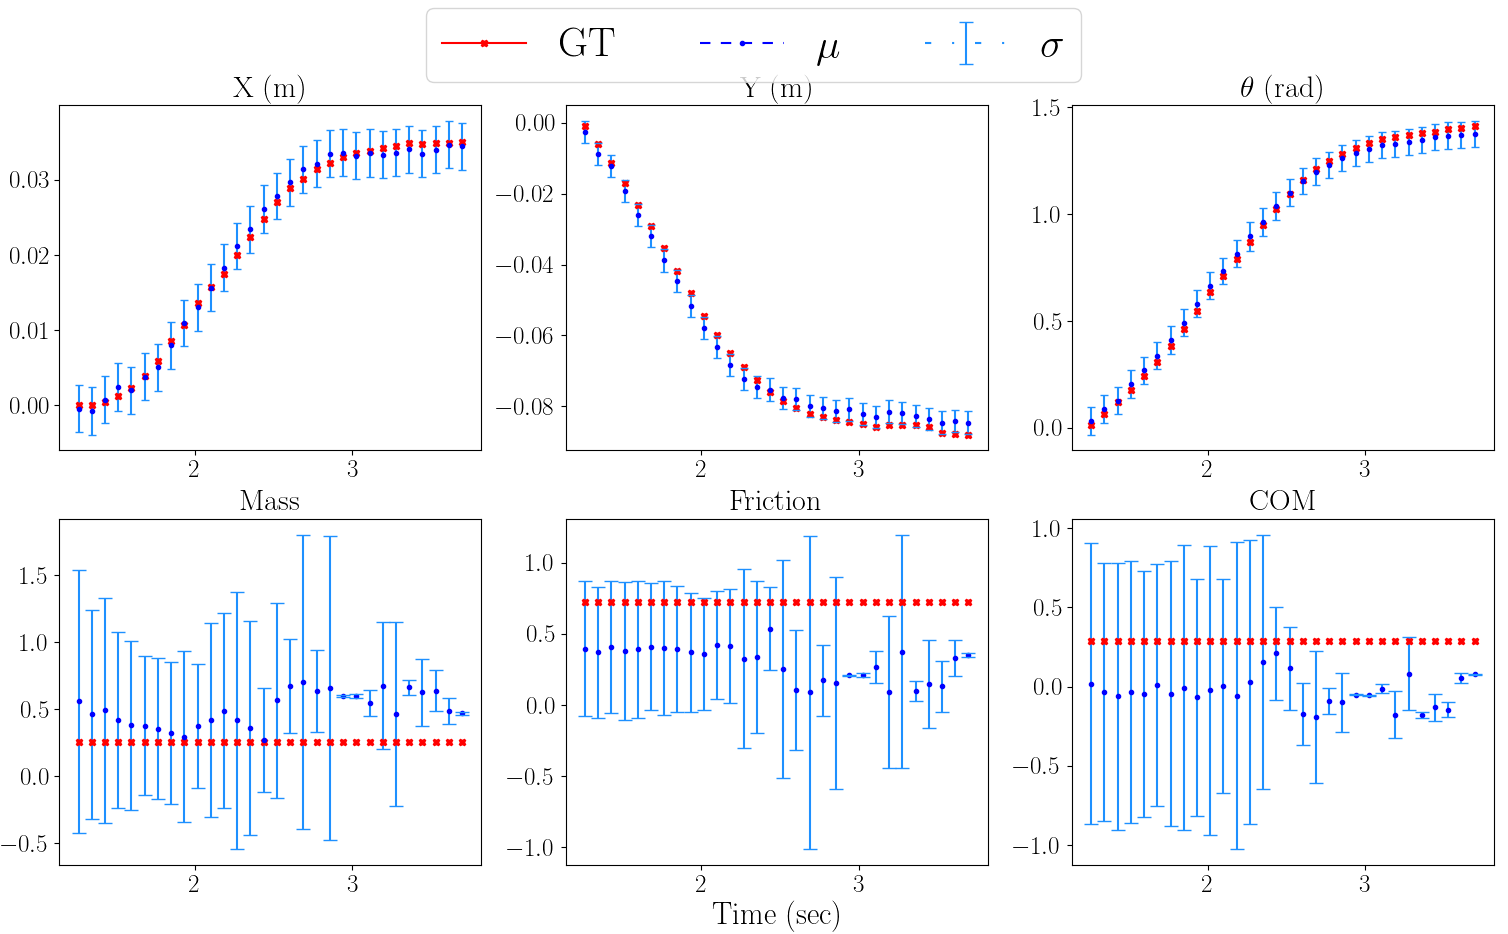}
    \caption{Filtering process for uniform object}
    \label{fig:filteringuniform}
\end{figure*}

\begin{figure*}[!tbh]
    \centering
    \includegraphics[width = \textwidth]{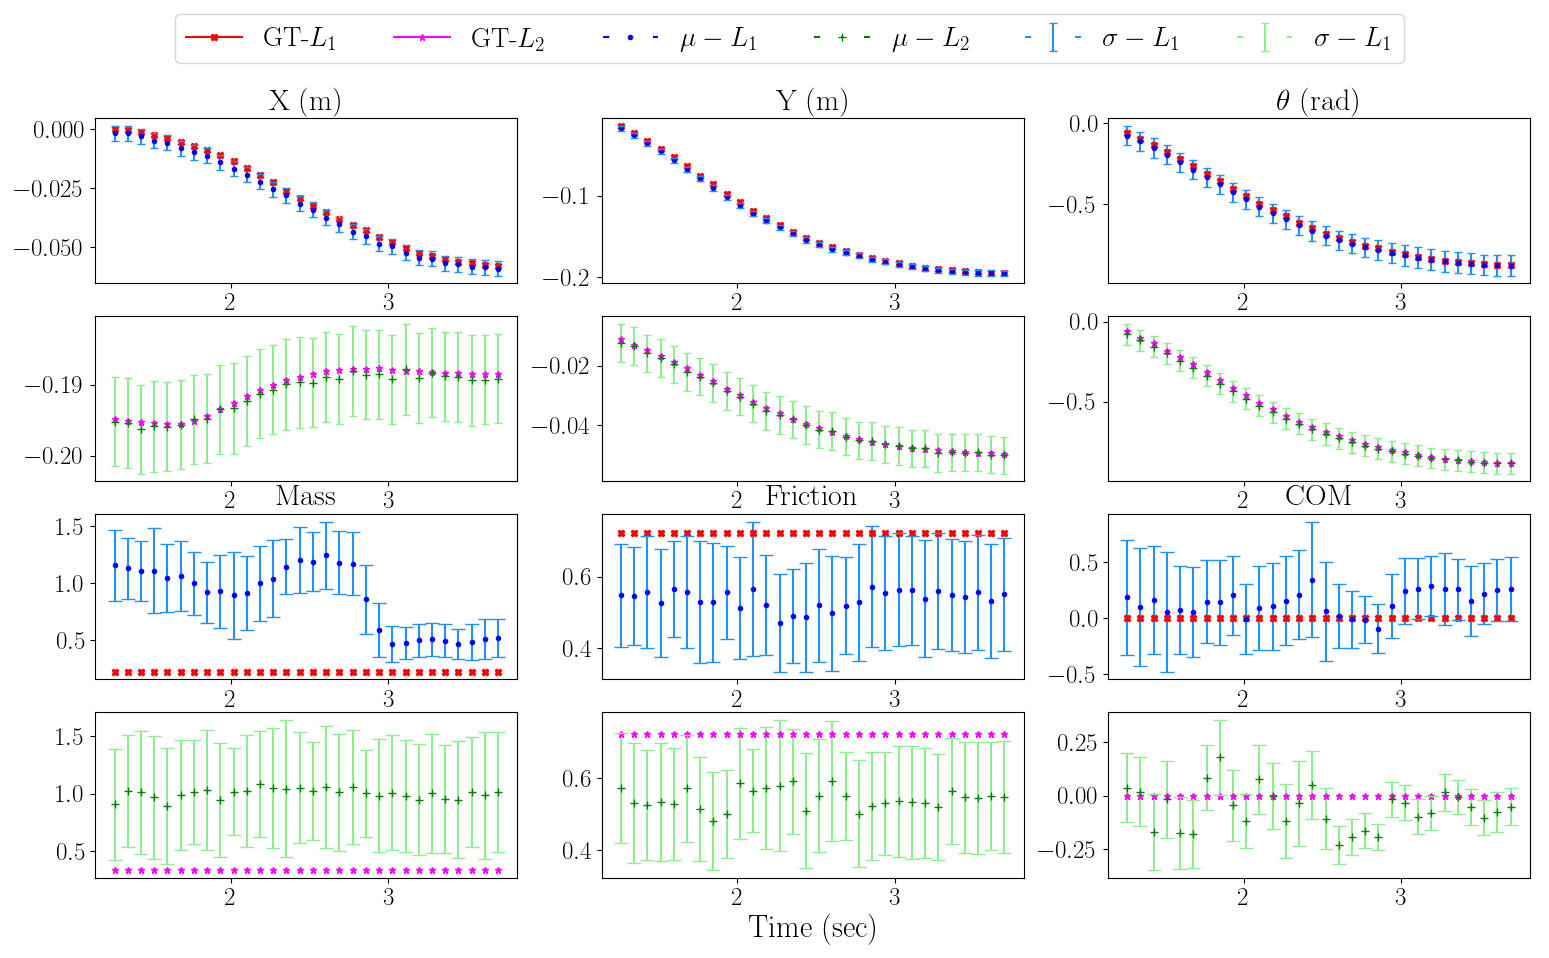}
    \caption{Filtering process for heterogeneous object with pushing}
    \label{fig:filteringheteropush}
\end{figure*}

\begin{figure*}[!tbh]
    \centering
    \includegraphics[width = \textwidth]{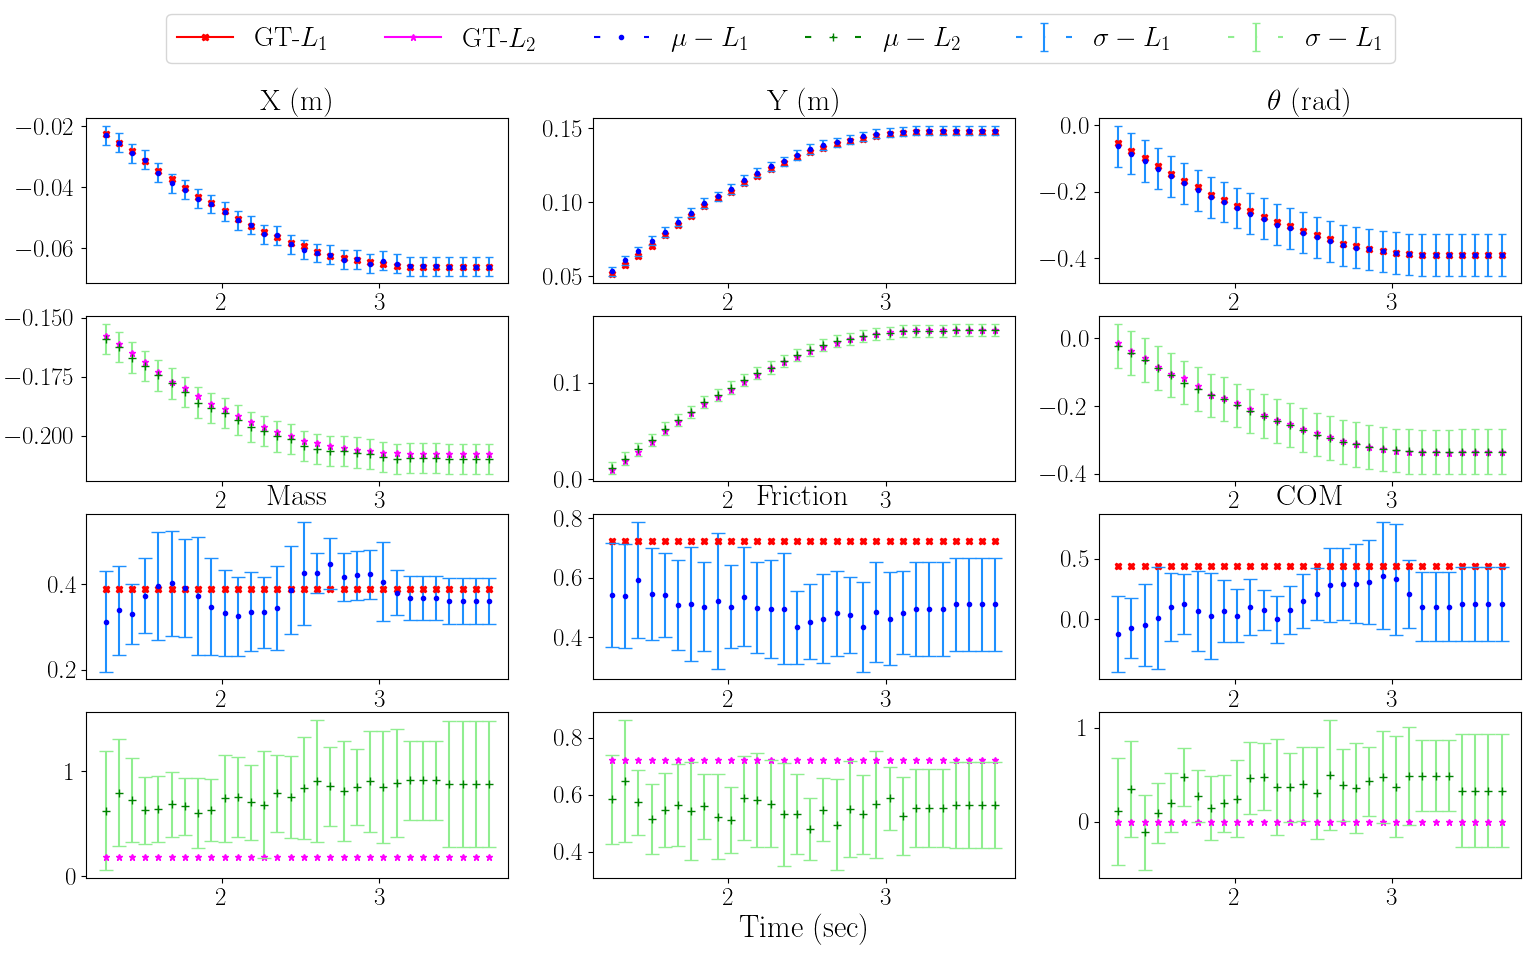}
    \caption{Filtering process for heterogeneous object with pulling}
    \label{fig:filteringheteropull}
\end{figure*}

\begin{figure*}[!tbh]
    \centering
    \includegraphics[width = \textwidth]{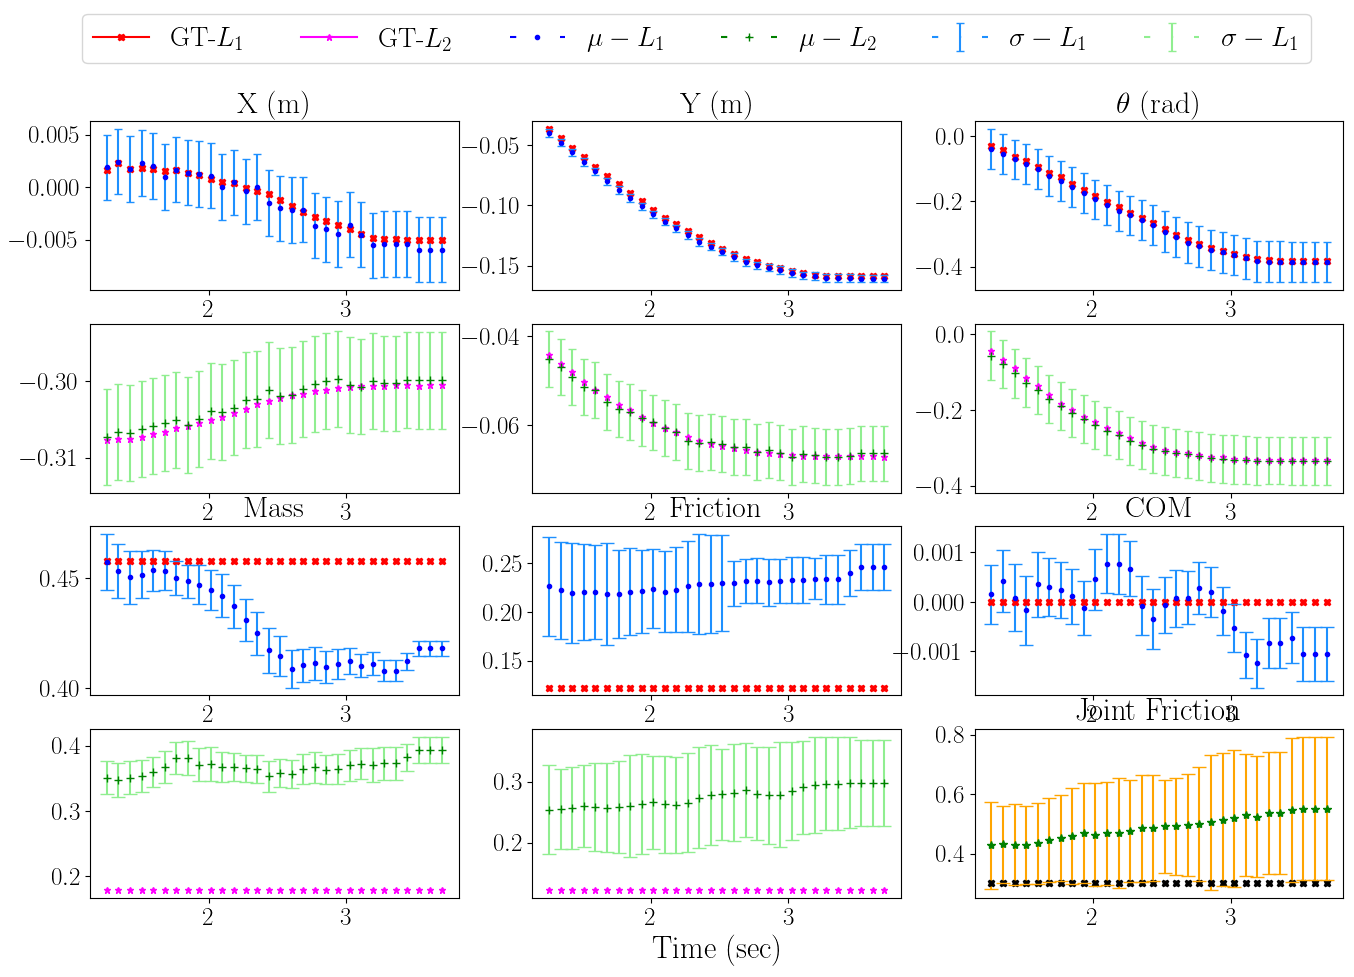}
    \caption{Filtering process for articulated object}
    \label{fig:filteringarticulatedpush}
\end{figure*}

\begin{figure*}[!tbh]
    \centering
    \includegraphics[width = \textwidth]{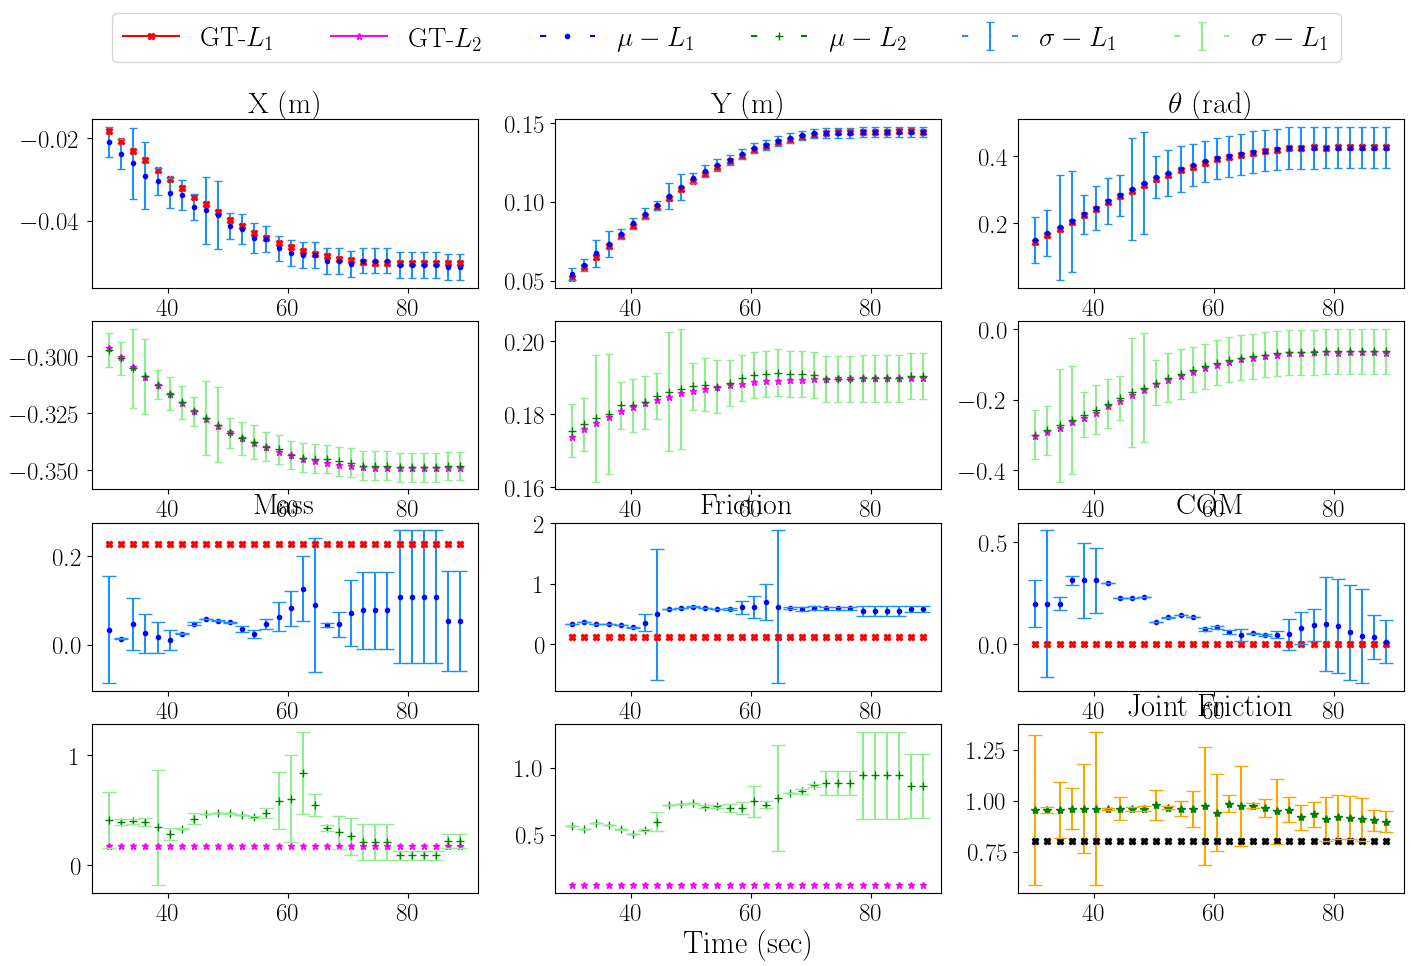}
    \caption{Inference results of articulated objects}
    \label{fig:filteringarticulatedpull}
\end{figure*}
